# Supplementary material for: Hierarchical Sparse Bayesian Multitask Learning for Disease Prediction in Pooled Microbiome Studies
Source: arXiv:2502.02552 source file (2026-09-21)
Supplement: Supplementary file 1 [file supp.tex]

\documentclass[journal,onecolumn]{IEEEtran}

\usepackage[utf8]{inputenc} % allow utf-8 input
\usepackage[T1]{fontenc}    % use 8-bit T1 fonts
\usepackage{hyperref}       % hyperlinks
\usepackage{url}            % simple URL typesetting
\usepackage{booktabs}       % professional-quality tables
\usepackage{amsfonts}       % blackboard math symbols
\usepackage{nicefrac}       % compact symbols for 1/2, etc.
\usepackage{microtype}      % microtypography
\usepackage{lipsum}
\usepackage{graphicx}
\usepackage{caption}
\usepackage{subcaption}
\usepackage{multirow}
\usepackage{amsmath, amssymb,amsthm}
\usepackage{color}
\usepackage{hyperref}
\usepackage{algorithm}
\usepackage{algpseudocode}
\usepackage{tikz}
\usepackage{longtable}
\usepackage{array}
\usepackage{geometry}
\usepackage{authblk}
\usetikzlibrary{fit,positioning}

\input{defs}

\graphicspath{ {./images/} }

\title{Supplementary: Hierarchical Bayesian Multitask Model for Microbiome Analysis}

\author[1,2, $\ast$]{Haonan Zhu}
\author[1,$\ast$]{Andre R. Goncalves}
\author[1]{Camilo Valdes}
\author[1]{Hiranmayi Ranganathan}
\author[1]{Boya Zhang}
\author[1]{Jose Manuel Martí}
\author[1]{Car Reen Kok}
\author[1]{Monica K. Borucki}
\author[1]{Nisha J. Mulakken}
\author[1]{James B. Thissen}
\author[1]{Crystal Jaing}
\author[2]{Alfred Hero}
\author[1, $\ast$]{Nicholas A. Be}

\affil[1]{Lawrence Livermore National Laboratory}
\affil[2]{Electrical and Computer Engineering, University of Michigan}
\affil[$\ast$]{Corresponding Authors: zhu18@llnl.gov, andre@llnl.gov, be1@llnl.gov} 

\begin{document} 
\maketitle

\section{Dataset References}

Table \ref{tab: dataset information} include references to all the studies used in this work along with their metadata. Some studies were obtained from the curatedMetagenomicData package \cite{pasolli2017accessible}.

\begin{longtable}{|>{\raggedright\arraybackslash}p{2.5cm}|p{1cm}|>{\raggedright\arraybackslash}p{2.5cm}|>{\raggedright\arraybackslash}p{2.5cm}|p{2.5cm}|}
\caption{Summary of microbiome studies by disease categories. Notably \cite{zysset2020associations} contains two diseases (age-related macular degeneration, cardiovascular disease) and \cite{mcdonald2018american} contains six diseases (diabetes, neurological disease, irritable bowel syndrome, inflammatory bowel disease, gastrointestinal infection and diarrhea, therefore they are split into multiple studies based on the disease categories for our analysis.} 
\label{tab: dataset information}\\
\hline 
\textbf{Disease Category} & \textbf{Ref.} & \textbf{Host Body Site} & \textbf{Geographic Location} & \textbf{Control and Disease Splits (C/D)} \\
\hline
\endfirsthead

\multicolumn{5}{c}%
{{\bfseries \tablename\ \thetable{} -- continued from previous page}} \\
\hline 
\textbf{Disease Category} & \textbf{Ref.} & \textbf{Host Body Site} & \textbf{Geographic Location} & \textbf{Control and Disease Splits (C/D)} \\
\hline
\endhead

\hline \multicolumn{5}{|r|}{{Continued on next page}} \\ \hline
\endfoot

\hline
\endlastfoot

\multirow{4}{1.7cm}{Diabetes} & \cite{karlsson2013gut} & Fecal & Europe & 43/102 \\
                              & \cite{sankaranarayanan2015gut} & Fecal & United States & 17/19 \\
                              & \cite{heintz2016integrated} & Fecal & Luxembourg & 26/27 \\
                              & \cite{mcdonald2018american} & Fecal & United States & 359/19 \\
\hline                                     
\multirow{2}{1.7cm}{Cirrhosis} & \cite{qin2014alterations} & Fecal & China & 113/110 \\
                               & \cite{loomba2019gut} & Fecal & United States & 77/9 \\
\hline                                     
\multirow{5}{1.7cm}{Cancer}    & \cite{feng2015gut} & Fecal & Austria & 61/93 \\
                               & \cite{yu2017metagenomic} & Fecal & China & 53/75 \\
                               & \cite{hannigan2018diagnostic} & Fecal & North America & 21/36 \\
                               & \cite{yachida2019metagenomic} & Fecal & Japan & 250/365 \\
                               & \cite{nagata2022metagenomic} & Fecal, Oral & Not Available & 470/90 \\
\hline                                     
\multirow{8}{1.7cm}{Neurological\\ Disease} & \cite{castro2015composition} & Oral & United States & 16/16 \\
                                           & \cite{nagy2017fecal} & Fecal & United States & 50/50 \\
                                           & \cite{qian2020gut} & Fecal & China & 40/40 \\
                                           & \cite{zhu2020metagenome} & Fecal & China & 81/90 \\
                                           & \cite{jo2022oral} & Fecal, Oral & South Korea & 74/81 \\
                                           & \cite{laske2022signature} & Fecal & Germany & 100/75 \\
                                           & \cite{wallen2022metagenomics} & Fecal & United States & 233/491 \\
                                           & \cite{mcdonald2018american} & Fecal & United States & 359/253 \\
\hline                                                    
\multirow{3}{1.7cm}{Diarrhea}  & \cite{david2015gut} & Fecal, Rectal Swab & Bangladesh & 7/23 \\
                               & \cite{kieser2018bangladeshi} & Fecal & Bangladesh & 9/18 \\
                               & \cite{mcdonald2018american} & Fecal & United States & 359/60 \\
\hline                      
\multirow{4}{1.7cm}{Dermatologic Disease} & \cite{chng2016whole} & Skin & Asia & 40/38 \\
                                          & \cite{byrd2017staphylococcus} & Skin & United States & 53/238 \\
                                          & \cite{tay2021atopic} & Skin & Singapore & 50/69 \\
                                          & \cite{chang2022multiomic} & Fecal & United States & 15/33 \\
\hline                                                    
\multirow{4}{1.7cm}{Gastrointestinal Infection} & \cite{vincent2016bloom} & Fecal & Canada & 182/27 \\
                                                & \cite{rosa2018differential} & Fecal & Indonesia, Liberia & 5/19 \\
                                                & \cite{rubel2020lifestyle} & Fecal & Cameroon & 86/89 \\
                                                & \cite{mcdonald2018american} & Fecal & United States & 359/5 \\
\hline                                              
\multirow{5}{1.7cm}{Inflammatory Bowel Disease} & \cite{hall2017novel} & Fecal & United States & 71/175 \\
                                                & \cite{franzosa2019gut} & Fecal & Not Available & 56/162 \\
                                                & \cite{integrative2014integrative} & Fecal & Not Available & 354/888 \\
                                                & \cite{zuo202216s} & Fecal & United States & 27/8 \\
                                                & \cite{mcdonald2018american} & Fecal & United States & 359/9 \\
\hline                                               
\multirow{6}{1.7cm}{Cardiovascular Disease} & \cite{jie2017gut} & Fecal & China & 171/214 \\
                                            & \cite{li2017gut} & Fecal & China & 41/155 \\
                                            & \cite{yan2017alterations} & Fecal & China & 56/60 \\
                                            & \cite{polster2020permissive} & Fecal & United States & 27/127 \\
                                            & \cite{xiong2022cerebral} & Fecal & China & 10/10 \\
                                            & \cite{zysset2020associations} & Fecal & Switzerland & 30/29 \\
\hline 
\multirow{3}{1.7cm}{Oral Disease} & \cite{espinoza2018supragingival} & Oral & Australia & 37/48 \\
                                  & \cite{ghensi2020strong} & Oral & Italy & 51/23 \\
                                  & \cite{wirth2022microbiomes} & Oral & Hungary & 8/19 \\
\hline 
\multirow{2}{1.7cm}{Autoimmune Disease} & \cite{ye2018metagenomic} & Fecal & China & 45/20 \\
                                        & \cite{zhu2021compositional} & Fecal & China & 62/100 \\
\hline
\pagebreak
\multirow{2}{1.7cm}{Immune Disease} & \cite{guillen2019low} & Fecal & Spain & 27/129 \\
                                    & & & & \\
\hline
\multirow{8}{1.7cm}{Pulmonary Disease} & \cite{hu2019gut} & Fecal & China & 31/46 \\
                                        & \cite{pust2020human} & Cough Swabs & Germany & 48/49 \\
                                        & \cite{zuo2020alterations} & Fecal & China & 15/55 \\
                                        & \cite{bai2022characterization} & Nasal & Sweden & 20/37 \\
                                        & \cite{liu2022gut} & Fecal & China & 63/47 \\
                                        & \cite{xiao2022insights} & Lung (Bronchioalveolar Lavage Fluid) & China & 16/45 \\
                                        & \cite{zhang2022prolonged} & Fecal & China & 69/138 \\
                                        & \cite{zhou2022sars} & Fecal & China & 21/20 \\
\hline
\multirow{2}{1.7cm}{Metabolic Disease} & \cite{maya2019gut} & Fecal & Mexico & 10/10 \\
                                       & & & & \\
\hline
\multirow{2}{1.7cm}{Hormonal  Disorder} & \cite{qi2019gut} & Fecal & China & 43/50 \\
                                        & & & & \\
\hline 
\multirow{3}{1.7cm}{Genitourinary Disease} & \cite{bommana2022metagenomic} & Endocervical, Vaginal, Rectal   & Fiji & 11/14 \\
                                        & &  & & \\
                                        & &  & & \\
\hline
\multirow{2}{1.7cm}{Seafaring Syndrome} & \cite{sun2022interactions} & Fecal & Not Available & 99/55 \\
              & & & & \\
\hline
\multirow{3}{1.7cm}{Irritable Bowel Syndrome} & \cite{mcdonald2018american} & Fecal & United States & 359/52 \\
              & & & & \\
              & & & & \\
\hline
\multirow{4}{1.7cm}{Age-Related Macular Degeneration} & \cite{zysset2020associations} & Fecal & Switzerland & 33/57 \\
              & & & & \\
              & & & & \\
              & & & & \\
\hline
\end{longtable}

\section{CAVI update derivation}
\label{sec: CAVI update derivation}

This section includes the derivations of CAVI updates for Algorithm I. 

Recall Equation 18 of \cite{blei2017variational} states that if we are to approximate a general posterior distribution $p\left(  \mb \xi \mid \text{data}  \right) $ with a mean-field approximation $q\left(  \mb \xi \right):=\prod_{j} q_{j}\left(\xi_{j} \right) $, the CAVI update for $j$-th latent variable $\xi_{j}$ (i.e., the optimal solution $q_{j}^{\star}\left( \xi_{j} \right) $) is proportional to the exponentiated conditional expected log of the joint:
\begin{equation}
\label{eqn: cavi update rule}
q^{\star}_{j} \propto \exp\left( \expect[\mb \xi_{-j}\sim q_{-j}]{\log\left( p\left( \xi_{j}, \mb \xi_{-j}  \mid  \text{data}  \right)  \right) } \right).	
\end{equation}
where $\mb \xi_{-j}$ corresponds to all but the $j$-th latent variable.  

\paragraph{Update for $\alpha, \beta$}

Based on Eqn. \ref{eqn: cavi update rule}, the exponentiated conditional expectation of all the parameters except $\theta$ up to a constant scaling factor:
\begin{align*}
	q^{\star} \left( \theta \right) & \propto \exp\left( \left(\alpha_0-1\right) \log\theta +\left( \beta_0-1 \right)\log\left( 1-\theta \right) \right) \\
     & \quad \exp\left(\left( \sum_{j} \phi_{j} \right) \log \theta + \left( d-\sum_{j} \phi_{j}\right) \log\left( 1-\theta \right)      \right) \\
					& = \exp\left( \left( \alpha_0-1+\sum_{j} \phi_{j} \right) \log\theta \right)\\
     & \quad \exp\left(\left( \beta_0+d-\sum_{j} \phi_{j} -1 \right) \log\left( 1-\theta \right)     \right).
\end{align*}

This implies $q^{\star}\left( \theta \right)$ follows a beta distribution with parameters:
\begin{align*}
	\alpha & = \alpha_0+\sum_{j} \phi_{j}, \\
	\beta & = \beta_0+d-\sum_{j} \phi_{j}.
\end{align*}

\paragraph{Update for $v$ and  $\mb V$} Based on Eqn. \ref{eqn: cavi update rule}, the exponentiated conditional expectation of all the parameters except $\mb \Sigma_{0}^{-1}$ up to a constant scaling factor:
 \begin{align*}
	 q^{\star}\left( \mb \Sigma_0^{-1} \right) & \propto \exp \left(-\frac{1}{2} \trace \left( \mb V_0^{-1}\mb \Sigma_0^{-1} \right) \right) \\
   &\quad \exp\left(-\frac{v_0+d-T-1}{2} \log\det\left( \mb \Sigma_0^{-1} \right) \right)\\
   &\quad \exp\left(- \frac{1}{2}\trace\left( \mb \Sigma_0^{-1} \left( \sum_{j} \mb m_{\left( j \right) } \mb m_{\left( j \right) }^{\top} + \mb \Sigma_{j} \right)  \right) \right).  
\end{align*}
This implies $q^{\star}\left( \mb \Sigma_{0}^{-1} \right)$ follow a Wishart distribution with parameters:
\begin{align*}
	v & = v_0+d, \\
	\mb V &=\left( \mb V_0^{-1}+\sum_{j} \mb m_{\left( j \right)} \mb m_{\left( j \right) }^{\top}+\mb \Sigma_{j} \right)^{-1}. 
\end{align*}
\paragraph{Update for $\mb \Sigma_{j}$}
all the terms involve $\mb \Sigma_{j}$ in ELBO approximation (Eqn. 3, section III.A):
\[
-\frac{1}{2}\trace\left( v \mb V \mb \Sigma_{j} \right)-\frac{1}{8} \sum_{t} \left( \mb \Sigma_{j} \right)_{t,t} \phi_{j}\sum_{i}\left( x_{t}^{ij} \right)^{2} +\frac{1}{2}\log\det\left( \mb \Sigma_{j} \right)  
.\] 
Rewrite the second term:
\[
-\frac{1}{8} \trace\left( \mb \Sigma_{j} \diag\left( \begin{bmatrix} \sum_{i} \phi_{j}\left(x_{1}^{ij} \right)^{2},\cdots, \sum_{i} \phi_{j}\left( x_{T}^{ij} \right)^{2}     \end{bmatrix}^{\top} \right)  \right) 
.\] 
Denote the diagonal matrix as $\tilde{\mb X_{j}}$. For every $j$, we have a constrained optimization problem:
\[
	\max_{\mb \Sigma \in \bb S_{++}^{T}} \log\det\left( \mb \Sigma \right)-\trace\left( \mb \Sigma \left(v \mb V+\frac{1}{4} \tilde{\mb X_{j}} \right)  \right)  
.\] 
which admits a closed form solution:
\begin{equation}
\label{eqn: covariance updates}
	\mb \Sigma_{j}^{\star} = \left( v \mb V + \frac{1}{4} \tilde{\mb X_{j}} \right)^{-1}. 
\end{equation}
for $j=1,\ldots, d$. 

\paragraph{Update for $\mb m_{\left( j \right) }$}
all the terms involved $\mb m_{\left( j \right) }$ in ELBO approximation (Eqn. 3, section III.A):
\begin{align*}
    %f\left(  \mb m_{\left( j \right) }\right) 
    & -\frac{v}{2} \innerprod{\mb m_{\left( j \right) }}{\mb V \mb m_{\left(j\right) }} -\frac{1}{8}\innerprod{\mb m_{\left( j \right) }}{\tilde{\mb X_{j}}\mb m_{\left( j \right) }}\\
    &+\innerprod{\mb m_{\left( j \right) }}{\begin{bmatrix} \cdots, & \phi_{j}\sum_{i} \left(y_{t}^{i}-\tilde{y_{t}^{i}}\right) x_{t}^{ij}, & \cdots\end{bmatrix}^{\top}}\\
    &+\frac{1}{4} \innerprod{\mb m_{\left( j \right) }}{\begin{bmatrix} \cdots, & \phi_{j} \sum_{i} \innerprod{\mb w'_{t} \circ \mb z'}{\mb x_{t}^{i}}x_{t}^{ij}, &\cdots \end{bmatrix}^{\top}}\\
    &-\frac{1}{4}\innerprod{\mb m_{\left( j \right) }}{\begin{bmatrix} \cdots, & \phi_{j}\sum_{i} x_{t}^{ij} \sum_{l\neq j} \phi_{l}x_{t}^{il} m_{tl}, &\cdots \end{bmatrix}^{\top} }.
\end{align*}
This problem is quadratic with a negative definite Hessian matrix, hence by stationary condition (i.e., zero gradient) we have closed form updates: 
\begin{align}
\label{eqn: genereal mean updates}
    & \mb \Sigma_{j}^{\star} ( \begin{bmatrix} \cdots & \phi_{j}\sum_{i} \left(y_{t}^{i}-\tilde{y_{t}^{i}}\right) x_{t}^{ij}, & \cdots\end{bmatrix}^{\top} \nonumber \\ 
    &\quad +\frac{1}{4} \begin{bmatrix} \cdots, & \phi_{j} \sum_{i} \innerprod{\mb w'_{t} \circ \mb z'}{\mb x_{t}^{i}}x_{t}^{ij}, &\cdots \end{bmatrix}^{\top} \nonumber \\
    &\quad -\frac{1}{4} \begin{bmatrix} \cdots, & \phi_{j}\sum_{i} x_{t}^{ij} \sum_{l\neq j} \phi_{l}x_{t}^{il} m_{tl}, &\cdots \end{bmatrix}^{\top} 
	). 
\end{align}
For all $j=1\ldots, d$. When the reference point of quadratic lower bound $\mb w' \circ \mb z'$ is set to be the mean parameters from the previous iteration, we can simplify Eqn. \ref{eqn: mean updates}:
{\small
\begin{align}
	\label{eqn: mean updates}	
	 & \mb \Sigma_{j}^{\star} ( \begin{bmatrix} \phi_{j}\sum_{i} \left(y_{1}^{i}-\tilde{y_{1}^{i}}\right) x_{1}^{ij}, & \cdots, & \phi_{j}\sum_{i} \left(y_{T}^{i}-\tilde{y_{T}^{i}}\right) x_{T}^{ij} \end{bmatrix}^{\top} \nonumber \\
     &\quad +\frac{1}{4} \begin{bmatrix} \phi_{j}^{2} \sum_{i} \left(x_{1}^{ij}\right)^{2} m_{1j}^{\left( k \right) }, &\cdots, & \phi_{j}^{2} \sum_{i} \left( x_{T}^{ij} \right)^{2} m_{Tj}^{\left( k \right) }  \end{bmatrix}^{\top}. \nonumber \\	
\end{align}
}
\paragraph{Update for $\phi_{j}$}

All the terms involve $\phi_{j}$ in ELBO approximation (Eqn. 3, section III.A): 
\begin{align*}
	f\left( \phi_{j} \right) &:= \phi_{j}\left( \psi\left( \alpha \right) -\psi\left( \beta \right) \right)   +\phi_{j}\sum_{t}\sum_{i} \left( y_{t}^{i}-\tilde{y_{t}^{i}}\right)m_{tj} x_{t}^{ij} \\
	%f\left( \phi_{j} \right) &:= \phi_{j}\left( \psi\left( \alpha \right) -\psi\left( \beta \right) +\psi\left( \alpha+\beta \right)  \right)   +\phi_{j}\sum_{t}\sum_{i} \left( y_{t}^{i}-\tilde{y_{t}^{i}}\right)m_{tj} x_{t}^{ij} \\
				 &\quad +\frac{\phi_{j}}{4} \sum_{t}\sum_{i} \left(m_{tj} x_{t}^{ij}\right) \innerprod{\mb w_{t}'\circ\mb z'}{\mb x_{t}^{i}}\\ 
				 &\quad -\frac{\phi_{j}}{4}\sum_{t}\sum_{i} m_{tj} x_{t}^{ij} \sum_{l\neq j} m_{tl} \phi_{l} x_{t}^{il}\\ 
     &\quad -\frac{\phi_{j}}{8}\sum_{t}\left( \left( \Sigma_{j} \right)_{tt}+m_{tj}^{2} \right)\sum_{i}\left( x_{t}^{ij} \right)^{2}  \\
				 & \quad -\phi_{j}\log\left( \phi_{j} \right)-\left( 1-\phi_{j} \right) \log\left( 1-\phi_{j} \right).  
\end{align*}
Observe $f\left( \phi_{j} \right)$ is a smooth strictly concave function, so we can solve for $\phi_{j}^{\star}$ by stationary condition (i.e., $0$ derivatives), which admit a closed form update:
 \begin{align}
\label{eqn: general sparsity updates}
\phi_{j}^{\star} &= \sigma\left( a \right).  	
\end{align}
where $\sigma\left( t \right):=\frac{1}{\exp\left( -t \right)+1}$ denote the sigmoid function, and: 
\begin{align*}
	 a & = \psi\left( \alpha \right) -\psi\left( \beta \right) + \sum_{t}\sum_{i} \left( y_{t}^{i}-\tilde{y_{t}^{i}}\right)m_{tj} x_{t}^{ij} \\
	 %a & = \psi\left( \alpha \right) -\psi\left( \beta \right) +\psi\left( \alpha+\beta \right) + \sum_{t}\sum_{i} \left( y_{t}^{i}-\tilde{y_{t}^{i}}\right)m_{tj} x_{t}^{ij} \\
        &\quad +\frac{1}{4} \sum_{t}\sum_{i} \left(m_{tj} x_{t}^{ij}\right) \innerprod{\mb w_{t}'\circ\mb z'}{\mb x_{t}^{i}}\\ 
        &\quad -\frac{1}{4}\sum_{t}\sum_{i} m_{tj} x_{t}^{ij} \sum_{l\neq j} m_{tl} \phi_{l} x_{t}^{il}\\
        & \quad -\frac{1}{8}\sum_{t}\left( \left( \Sigma_{j} \right)_{tt}+m_{tj}^{2} \right)\sum_{i}\left( x_{t}^{ij} \right)^{2}.  \\
\end{align*}

When reference point of quadratic lower bound $\mb w' \circ \mb z'$ is set to be the mean parameters from the previous iterations, Eqn. \ref{eqn: general sparsity updates} is simplified: 
\begin{align}
\label{eqn: sparsity updates}
\phi_{j}^{k+1} &= \sigma\left( a\right).	
\end{align}
where 
\begin{align*}
	 a & = \psi\left( \alpha \right) -\psi\left( \beta \right)  + \sum_{t}\sum_{i} \left( y_{t}^{i}-\tilde{y_{t}^{i}}\right)m_{tj} x_{t}^{ij} \\
	 %a & = \psi\left( \alpha \right) -\psi\left( \beta \right) +\psi\left( \alpha+\beta \right) + \sum_{t}\sum_{i} \left( y_{t}^{i}-\tilde{y_{t}^{i}}\right)m_{tj} x_{t}^{ij} \\
	   &+\frac{1}{8}\sum_{t}\left(  m_{tj}^{2}\left(2\phi_{j}^{\left( k \right) }-1\right)-\left( \Sigma_{j} \right)_{tt}  \right)\sum_{i}\left( x_{t}^{ij} \right)^{2} .
\end{align*}

\section{Additional Experimental Results}
\label{sec: additional exp results}

This section includes additional experimental results.  We exam the methods using more evaluation metrics including: accuracy, balanced accuracy, averaged precision, F1 score, F2 score, and Matthews correlation coefficient (MCC). Table \ref{tab: bmtl eval metrics} summarizes the definitions of these metrics.
\begin{table}[htbp]
\renewcommand{\arraystretch}{1.25} % Increase row height
\small
\setlength{\tabcolsep}{4pt} % Adjust column separator width
\centering
\begin{tabular}{|p{2.5cm}|p{5.7cm}|} % Adjust column widths as needed
\hline
\textbf{Metric} & \textbf{Definition} \\
\hline
\text{TP} & \( \sum_{i=1}^{N} \mathbf{1}(y_i = 1 \land \hat{y}_i = 1) \) \\
\hline
\text{TN} & \( \sum_{i=1}^{N} \mathbf{1}(y_i = 0 \land \hat{y}_i = 0) \) \\
\hline
\text{FP} & \( \sum_{i=1}^{N} \mathbf{1}(y_i = 0 \land \hat{y}_i = 1) \) \\
\hline
\text{FN} & \( \sum_{i=1}^{N} \mathbf{1}(y_i = 1 \land \hat{y}_i = 0) \) \\
\hline
\text{Precision} & \( \frac{\text{TP}}{\text{TP} + \text{FP}} \) \\
\hline
\text{Recall} & \( \frac{\text{TP}}{\text{TP} + \text{FN}} \) \\
\hline
\text{Accuracy} & \( \frac{\text{TP} + \text{TN}}{N} \) \\
\hline
\text{Balanced Accuracy} & \( \frac{1}{2} \left( \frac{\text{TP}}{\text{TP} + \text{FN}} + \frac{\text{TN}}{\text{TN} + \text{FP}} \right) \) \\
\hline
%\text{Avg. Precision} & Integral of precision over all recall levels \\
%\hline
\text{F1 Score} & \( \frac{2 \cdot \text{Precision} \cdot \text{Recall}}{\text{Precision} + \text{Recall}} \) \\
\hline
\text{F2 Score} & \( \frac{5 \cdot \text{Precision} \cdot \text{Recall}}{4 \cdot \text{Precision} + \text{Recall}} \) \\
\hline
\text{MCC} & \( \frac{(\text{TP} \cdot \text{TN}) - (\text{FP} \cdot \text{FN})}{\sqrt{(\text{TP}+\text{FP})(\text{TP}+\text{FN})(\text{TN}+\text{FP})(\text{TN}+\text{FN})}} \) \\
\hline
\end{tabular}
\caption{Definitions of classification metrics and the intermediate variables given ground truth labels \( \mathbf{y} \) and predicted labels \( \hat{\mb y} \). \( \land \) denotes the "and" operation, and \( \mathbf{1}( \cdot ) \) is the indicator function, which is 11 if the condition inside is true and 0 otherwise.}
\label{tab: bmtl eval metrics}
\end{table}

\subsection{Synthetic Datasets}

This subsection include the detailed experimental results on the synthetic datasets summarized in Table \ref{tab:simulated support recovery}

\begin{table}[htbp]
	\centering
        \resizebox{0.95\columnwidth}{!}{
	\begin{tabular}{|p{1.7cm}|c|c|c|c|c|c|}
    	\hline
    	Dataset  & Metrics & BayesMTL & MTFL  & MSSL & STL-LC & Pooled-LC \\ 
    	\hline
    	\multirow{6}{4em}{dataset1 \\ (dense, \\balanced)} & Accuracy & 0.322 (0.06) & \textbf{0.793} (0.05) & \textbf{0.793} (0.05) & 0.688 (0.05) & 0.71 (0.04) \\ 
    	& Balanced Accuracy & \textbf{0.565} (0.03) & 0.5 (0) & 0.5 (0) & 0.525 (0.05) & 0.52 (0.03) \\
    	& Average Precision  & \textbf{0.819} (0.05) & 0.793 (0.05) & 0.793 (0.05) & 0.803 (0.04) & 0.800 (0.05) \\
    	& F1 Score  & 0.261 (0.06) & \textbf{0.884} (0.03)  & \textbf{0.884} (0.03) & 0.801 (0.04) & 0.821 (0.03) \\
    	& F2 Score  & 0.183 (0.05) & \textbf{0.950} (0.01) & \textbf{0.950} (0.01) & 0.800 (0.05) & 0.834 (0.03) \\
    	% & AUC  & \textbf{0.565} (0.03) & 0.5 (0) & 0.5 (0) & 0.525 (0.05) & 0.520 (0.03) \\
    	& MCC  & \textbf{0.156} (0.06) & 0 (0) & 0 (0) & 0.0565 (0.09) & 0.0427 (0.07)  \\
    	\hline
    	\multirow{6}{4em}{dataset2 \\ (sparse, \\balanced)} & Accuracy & \textbf{0.882} (0.04) & 0.225 (0.03) & 0.225 (0.03) & 0.438 (0.08) & 0.364 (0.02) \\ 
    	& Balanced Accuracy & \textbf{0.768} (0.05) & 0.5 (0) & 0.5 (0) & 0.616 (0.05) & 0.548 (0.04) \\
    	& Average Precision  & \textbf{0.597} (0.10) & 0.225 (0.03) & 0.225 (0.03) & 0.279 (0.06) & 0.244 (0.02) \\
    	& F1 Score  & \textbf{0.681} (0.09) & 0.367 (0.03) & 0.367 (0.03) & 0.431 (0.07) & 0.383 (0.03) \\
    	& F2 Score  & 0.602 (0.09) & 0.590 (0.03) & 0.590 (0.03) & \textbf{0.634} (0.06) & 0.579 (0.04) \\
    	% & AUC  & \textbf{0.768} (0.05) & 0.5 (0) & 0.5 (0) & 0.616 (0.05) & 0.548 (0.04) \\
    	& MCC  & \textbf{0.638} (0.10) & 0 (0) & 0 (0) & 0.227 (0.09) & 0.104 (0.07) \\
    	\hline
    	\multirow{6}{4em}{dataset3 \\ (ultra sparse, \\ balanced)}  & Accuracy & \textbf{0.988} (0.02) & 0.0350 (0.01) & 0.0350 (0.01) & 0.437 (0.08) & 0.199 (0.04)\\ 
    	& Balanced Accuracy & \textbf{0.947} (0.06) & 0.5 (0) & 0.5 (0) & 0.708 (0.04) & 0.526 (0.09) \\
    	& Average Precision  & \textbf{0.801} (0.20)& 0.035 (0.01)& 0.035 (0.01)& 0.0584 (0.01) & 0.0372 (0.01) \\
    	& F1 Score  & \textbf{0.876} (0.13) & 0.0674 (0.02) & 0.0674 (0.02) & 0.110 (0.02) & 0.070 (0.02) \\
    	& F2 Score  & \textbf{0.886} (0.12) & 0.152 (0.04) & 0.152 (0.04) & 0.235 (0.05) & 0.154 (0.04) \\
    	% & AUC  & \textbf{0.947} (0.06) & 0.5 (0) & 0.5 (0) & 0.708 (0.04) & 0.526 (0.09) \\
    	& MCC  & \textbf{0.879} (0.13) & 0 (0) & 0 (0) & 0.154 (0.02) & 0.0199 (0.08) \\
    	\hline 
    	\multirow{6}{4em}{dataset4 \\ (dense, \\ unbalanced)} & Accuracy & 0.441 (0.12) & \textbf{0.795} (0.04) & \textbf{0.795} (0.04) & 0.689 (0.09) & 0.693 (0.04)\\ 
    	& Balanced Accuracy & \textbf{0.584} (0.06) & 0.5 (0) & 0.5 (0) & 0.554 (0.07) & 0.517 (0.04) \\
    	& Average Precision  & \textbf{0.827} (0.04)& 0.795 (0.04) & 0.795 (0.04) & 0.814 (0.04) & 0.801 (0.04) \\
    	& F1 Score  & 0.483 (0.16) & \textbf{0.885} (0.02) & \textbf{0.885} (0.02) & 0.794 (0.08) & 0.808 (0.03) \\
    	& F2 Score  & 0.393 (0.15) & \textbf{0.951} (0.01) & \textbf{0.951} (0.01) & 0.788 (0.12) & 0.813 (0.04)\\
    	% & AUC  & \textbf{0.584} (0.06 )& 0.5 (0) & 0.5 (0) & 0.554 (0.07) & 0.517 (0.04)\\
    	& MCC  & \textbf{0.147} (0.09) & 0 (0) & 0 (0) & 0.118 (0.12) & 0.039 (0.08) \\
    	\hline
    	\multirow{6}{4em}{dataset5 \\ (sparse, \\unbalanced)} & Accuracy & \textbf{0.796} (0.07 )& 0.219 (0.04) & 0.219 (0.04) & 0.451 (0.07) & 0.334 (0.03)\\ 
    	& Balanced Accuracy & \textbf{0.783} (0.06) & 0.5 (0) & 0.5 (0) & 0.626 (0.036) & 0.541 (0.04)\\
    	& Average Precision  & \textbf{0.472} (0.13) & 0.219 (0.04) & 0.219 (0.04) & 0.275 (0.05) & 0.234 (0.03) \\
    	& F1 Score  & \textbf{0.625} (0.1) & 0.358 (0.05) & 0.358 (0.05) & 0.427 (0.06) & 0.370 (0.04) \\
    	& F2 Score  & \textbf{0.694} (0.05) & 0.579 (0.06) & 0.579 (0.06) & 0.630 (0.05) & 0.569 (0.04) \\
    	% & AUC  & \textbf{0.783} (0.06) & 0.5 (0) & 0.5 (0) & 0.626 (0.04) & 0.541 (0.04) \\
    	& MCC  & \textbf{0.516} (0.13) & 0 (0) & 0 (0) & 0.240 (0.05) & 0.086 (0.08)\\
    	\hline
    	\multirow{6}{4em}{dataset6 \\ (ultra sparse, \\ unbalanced)} & Accuracy & \textbf{0.917} (0.10) & 0.059 (0.0239) & 0.059 (0.0239) & 0.478 (0.07) & 0.21 (0.04) \\ 
    	& Balanced Accuracy & \textbf{0.905} (0.08) & 0.5 (0) & 0.5 (0) & 0.715 (0.05) & 0.553 (0.03)\\
    	& Average Precision  & \textbf{0.598} (0.02) & 0.059 (0.02) & 0.059 (0.02) & 0.097 (0.03) & 0.0646 (0.02) \\
    	& F1 Score  & \textbf{0.699} (0.27) & 0.11 (0.04) & 0.11 (0.04) & 0.176 (0.05)& 0.120 (0.04) \\
    	& F2 Score  & \textbf{0.763} (0.20) & 0.233 (0.08) & 0.233 (0.08) & 0.343 (0.08) & 0.246 (0.07) \\
    	% & AUC  & \textbf{0.905} (0.08) & 0.5 (0) & 0.5 (0) & 0.715 (0.05) & 0.553 (0.03) \\
    	& MCC  & \textbf{0.704} (0.26) & 0 (0) & 0 (0) & 0.198 (0.03) & 0.063 (0.03) \\
    	\hline
    \end{tabular}
    }
    \caption{Summary of the support recovery results for the simulated data. The bold number means the corresponding method is the best performing algorithm for the given metrics and dataset, and the values in parentheses represent standard deviations computed over $10$ different runs. The proposed Bayesian approach outperforms the benchmark methods in all evaluation metrics when there is a shared sparsity structure across regression coefficients of different tasks. Both MSSL and MTFL prioritize the prediction performance in the cross-validation step which results in complete dense solutions (i.e all regression coefficients are non-zero), hence they have identical results.}
    \label{tab:simulated support recovery}
\end{table}

\subsection{Microbiome Data}

This subsection include the additional experimental results on the microbiome data: table \ref{tab: microbiome prediction} includes the evaluations of the prediction performance, 
Fig. \ref{fig: traing predicted probability} and Fig. \ref{fig: test predicted probability} include the predicted probabilities on training and test data for the other taxonomic ranks respectively, Fig. \ref{fig: calibration curves} includes the additional calibration curves.

    \begin{table}[htbp]
    \centering
    \resizebox{\columnwidth}{!}{
    \begin{tabular}{|p{2cm}|c|c|c|c|c|c|}
        \hline 
          Taxon Ranks &            Metrics &    BayesMTL &          MTFL &             MSSL &       Pooled-LC &           STL-LC \\
        \hline
        \multirow{7}{4em}{Kingdom} &          Accuracy &0.681 (0.00956) &  \bf{0.685} (0.0116) &   \bf{0.685} (0.0121) & 0.532 (0.00974) &  0.618 (0.00725) \\
         &     Average Precision &  0.572 (0.00897) & 0.578 (0.00981) &  \bf{0.582} (0.00999) & 0.542 (0.00297) &   0.57 (0.00872) \\
         & Balanced Accuracy & 0.578 (0.0131) &  0.581 (0.0124) &   \bf{0.589} (0.0137) & 0.531 (0.00856) &   0.584 (0.0105) \\
        &           F1 Score &   0.588 (0.0163) &  0.587 (0.0147) &    \bf{0.59} (0.0121) &  0.474 (0.0106) &   0.523 (0.0284) \\
        &           F2 Score &   \bf{0.602} (0.0182) &  0.598 (0.0126) &   0.598 (0.0104) &  0.489 (0.0116) &   0.547 (0.0365) \\
        &               mcc &   0.171 (0.0281) &  0.178 (0.0309) &    \bf{0.19} (0.0345) & 0.0622 (0.0169) &   0.157 (0.0217) \\
         &     Sparsity Ratio &   0.288 (0.0102) &  0.541 (0.0298) &   0.467 (0.0267) &  0.883 (0.0408) &   \bf{0.263} (0.0203) \\
         \hline 
        \multirow{7}{4em}{Phylum} &          Accuracy & 0.689 (0.0178) &  \bf{0.715} (0.0159) &   0.701 (0.0174) & 0.552 (0.00715) &     0.655 (0.01) \\
          &     Average Precision &  0.598 (0.00862) & 0.615 (0.00804) &  \bf{0.621} (0.00927) & 0.538 (0.00385) &  0.593 (0.00802) \\
          & Balanced Accuracy & 0.618 (0.0146) &   0.64 (0.0147) &   \bf{0.651} (0.0151) &  0.527 (0.0085) &  0.612 (0.00993) \\
          &           F1 Score &   0.614 (0.0153) &    \bf{0.63} (0.018) &   0.627 (0.0158) & 0.521 (0.00613) &   0.579 (0.0387) \\
          &           F2 Score &   0.619 (0.0203) &   \bf{0.63} (0.0222) &   0.619 (0.0193) & 0.536 (0.00786) &   0.601 (0.0431) \\
          &               mcc &   0.243 (0.0309) &   0.294 (0.033) &    \bf{0.302} (0.033) & 0.0458 (0.0139) &   0.222 (0.0223) \\
          &     Sparsity Ratio &   0.182 (0.0169) & 0.301 (0.00222) &  0.311 (0.00286) &  0.781 (0.0247) &   \bf{0.0856} (0.012) \\
          \hline
          \multirow{7}{4em}{Class} &          Accuracy &0.688 (0.00922) &  \bf{0.726} (0.0099) &   0.695 (0.0156) &   0.58 (0.0163) &    0.668 (0.013) \\
           &     Average Precision &   0.599 (0.0107) & \bf{0.625} (0.00884) &   0.623 (0.0116) &  0.548 (0.0061) &  0.605 (0.00575) \\
           & Balanced Accuracy &  0.619 (0.013) &  \bf{0.659} (0.0114) &   0.656 (0.0167) &  0.544 (0.0121) &  0.629 (0.00728) \\
           &           F1 Score &   0.619 (0.0143) &  \bf{0.652} (0.0134) &    0.632 (0.016) &   0.54 (0.0155) &   0.584 (0.0269) \\
           &           F2 Score &   0.624 (0.0167) &  \bf{0.657} (0.0155) &   0.625 (0.0188) &  0.552 (0.0159) &    0.603 (0.037) \\
           &               mcc &   0.245 (0.0261) &  \bf{0.326} (0.0237) &   0.307 (0.0324) &  0.0803 (0.031) &    0.26 (0.0151) \\
           &     Sparsity Ratio &   0.116 (0.0121) &  0.24 (0.00565) &   0.295 (0.0531) &   0.692 (0.019) & \bf{0.0697} (0.00536) \\
          \hline 
          \multirow{7}{4em}{Order} &          Accuracy &   0.698 (0.01) &  \bf{0.703} (0.0116) &     0.68 (0.012) &   0.6 (0.00926) &    0.68 (0.0142) \\
           &     Average Precision &  0.609 (0.00955) & 0.618 (0.00827) &  \bf{0.622} (0.00906) &  0.558 (0.0044) &  0.617 (0.00803) \\
           & Balanced Accuracy & 0.634 (0.0126) &  0.655 (0.0123) &   \bf{0.659} (0.0131) & 0.557 (0.00793) &   0.645 (0.0119) \\
           &           F1 Score &  0.629 (0.00964) &   \bf{0.649} (0.018) &   0.623 (0.0202) &  0.553 (0.0147) &   0.574 (0.0121) \\
           &           F2 Score &   0.633 (0.0112) &  \bf{0.659} (0.0238) &   0.618 (0.0269) &  0.566 (0.0169) &   0.589 (0.0171) \\
           &               mcc &   0.271 (0.0234) &  \bf{0.309} (0.0279) &   0.306 (0.0237) &  0.112 (0.0148) &     0.29 (0.023) \\
           &     Sparsity Ratio &   0.109 (0.0115) & 0.199 (0.00967) &  0.222 (0.00103) & 0.536 (0.00935) &  \bf{0.046} (0.00772) \\
        \hline 
        \multirow{7}{4em}{Family} &          Accuracy & 0.704 (0.0218) &  0.687 (0.0148) &    0.665 (0.014) &  0.608 (0.0162) &  \bf{0.706} (0.00802) \\
          &     Average Precision &   0.613 (0.0168) &  0.625 (0.0144) &   0.621 (0.0145) &  0.567 (0.0104) &  \bf{0.632} (0.00636) \\
          & Balanced Accuracy & 0.643 (0.0256) &  0.658 (0.0149) &   0.656 (0.0139) &   0.57 (0.0179) &  \bf{0.663} (0.00637) \\
          &           F1 Score &   0.627 (0.0239) &   0.62 (0.0171) &   0.616 (0.0123) &  0.565 (0.0172) &   \bf{0.632} (0.0184) \\
          &           F2 Score &   0.631 (0.0235) &  0.609 (0.0223) &   0.612 (0.0126) &  0.574 (0.0164) &   \bf{0.648} (0.0183) \\
          &               mcc &   0.285 (0.0516) &  0.307 (0.0286) &   0.298 (0.0279) &  0.134 (0.0366) &  \bf{0.326} (0.00791) \\
          &     Sparsity Ratio &  0.0429 (0.0151) &   0.409 (x0.293) &  0.172 (0.00179) & 0.414 (0.00336) & \bf{0.0407} (0.00736) \\
          \hline 
          \multirow{7}{4em}{Genus} &          Accuracy & 0.707 (0.00852) &   0.65 (0.0291) &    0.66 (0.0156) & 0.619 (0.00865) &   \bf{0.728} (0.0158) \\
           &     Average Precision &  0.616 (0.00589) x&  0.609 (0.0168) &    0.62 (0.0123) & 0.575 (0.00737) &  \bf{0.647} (0.00831) \\x
           & Balanced Accuracy & 0.641 (0.0109) &  0.642 (0.0238) &   0.657 (0.0135) &  0.593 (0.0123) &  \bf{0.683} (0.00959) \\
           &           F1 Score &  0.634 (0.00774) &   0.562 (0.109) &   0.612 (0.0143) &  0.579 (0.0167) &   \bf{0.638} (0.0267) \\
           &           F2 Score &  0.638 (0.00785) &    0.562 (0.11) &     0.61 (0.015) &  0.589 (0.0219) &   \bf{0.649} (0.0305) \\
           &               mcc &   0.288 (0.0204) &  0.272 (0.0468) &     0.3 (0.0265) &  0.175 (0.0246) &     \bf{0.366} (0.02) \\
           &     Sparsity Ratio & \bf{0.0181} (0.00677) &   0.403 (0.281) &  0.152 (0.00116) & 0.326 (0.00331) & 0.0351 (0.00621) \\
           \hline 
        \multirow{7}{4em}{Species} &          Accuracy & 0.711 (0.0143) &   0.57 (0.0205) &   0.672 (0.0106) &  0.648 (0.0113) &   \bf{0.744} (0.0145) \\
         &     Average Precision &    0.621 (0.015) &  0.57 (0.00941) &  0.628 (0.00825) & 0.593 (0.00687) &    \bf{0.66} (0.0119) \\
         & Balanced Accuracy &  0.65 (0.0168) &  0.584 (0.0158) &   0.671 (0.0117) &  0.626 (0.0103) &    \bf{0.7} (0.0132) \\
         &           F1 Score &   0.635 (0.0168) &  0.301 (0.0674) &   0.622 (0.0108) & 0.611 (0.00954) &   \bf{0.651} (0.0222) \\
         &           F2 Score &   0.634 (0.0146) &  0.297 (0.0656) &   0.618 (0.0136) &  0.625 (0.0128) &   \bf{0.661} (0.0244) \\
         &               mcc &   0.305 (0.0333) &   0.16 (0.0288) &    0.325 (0.023) &  0.234 (0.0202) &   \bf{0.401} (0.0279) \\
         &     Sparsity Ratio &  \bf{0.0289} (0.0053) &  0.149 (0.0275) & 0.149 (0.000836) & 0.279 (0.00367) & 0.0319 (0.00481) \\
        \hline 
        \end{tabular}
        }
	   \caption{Summary of the prediction performance. The bold number means the corresponding method is the best performing algorithm for the given metrics and taxonomic rank, and the values in parentheses represent standard deviations computed over $5$ different runs. Due to the heterogeneous nature of the data, we do not see an improvement of the proposed approach over single-tasked model. However, the proposed approach is the only multitask method that provides a sparse solution i.e identify common bacteria across studies of the same disease categories that are informative for the predictions.}
	\label{tab: microbiome prediction}
\end{table}

\begin{figure}[htbp]
	\centering
	\begin{subfigure}{0.3\columnwidth}
        	\centering
		\includegraphics[width=\textwidth]{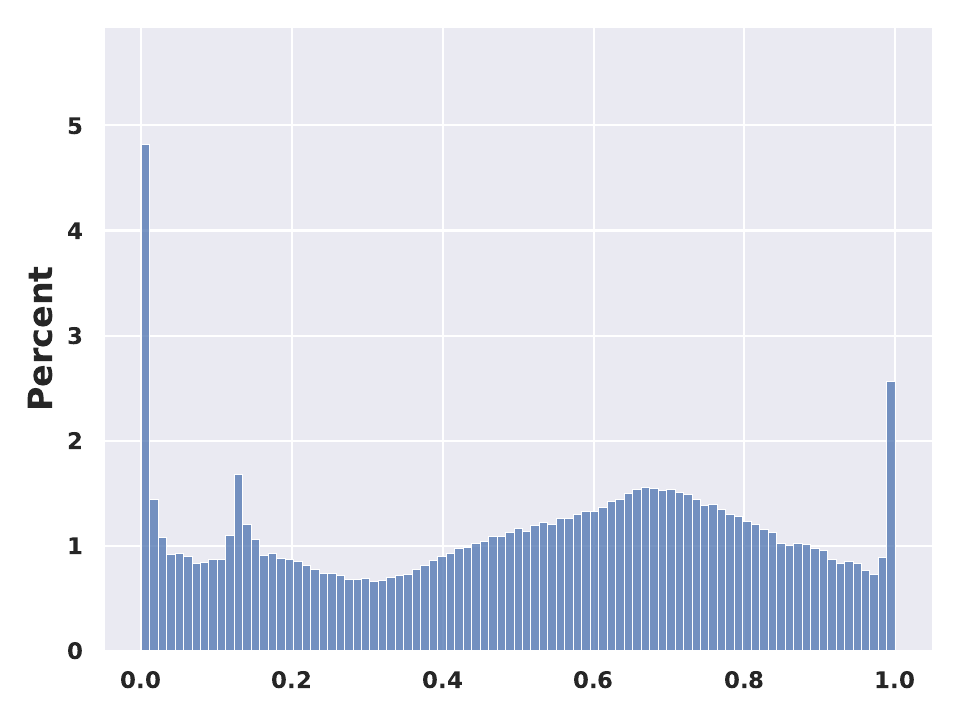}
		\caption{Kingdom}
		\label{subfig: y_pred_train predict Kingdom}
	\end{subfigure}
	\begin{subfigure}{0.3\columnwidth}
        	\centering
		\includegraphics[width=\textwidth]{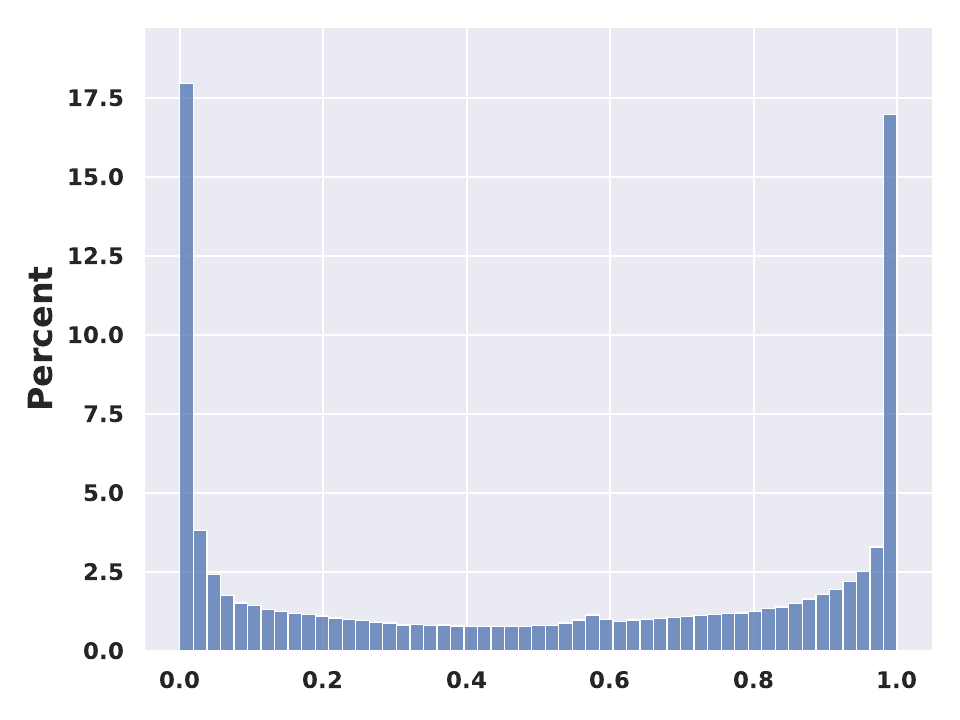}
		\caption{Phylum}
		\label{subfig: y_pred_train predict Phylum}
	\end{subfigure}
	\begin{subfigure}{0.3\columnwidth}
        	\centering
		\includegraphics[width=\textwidth]{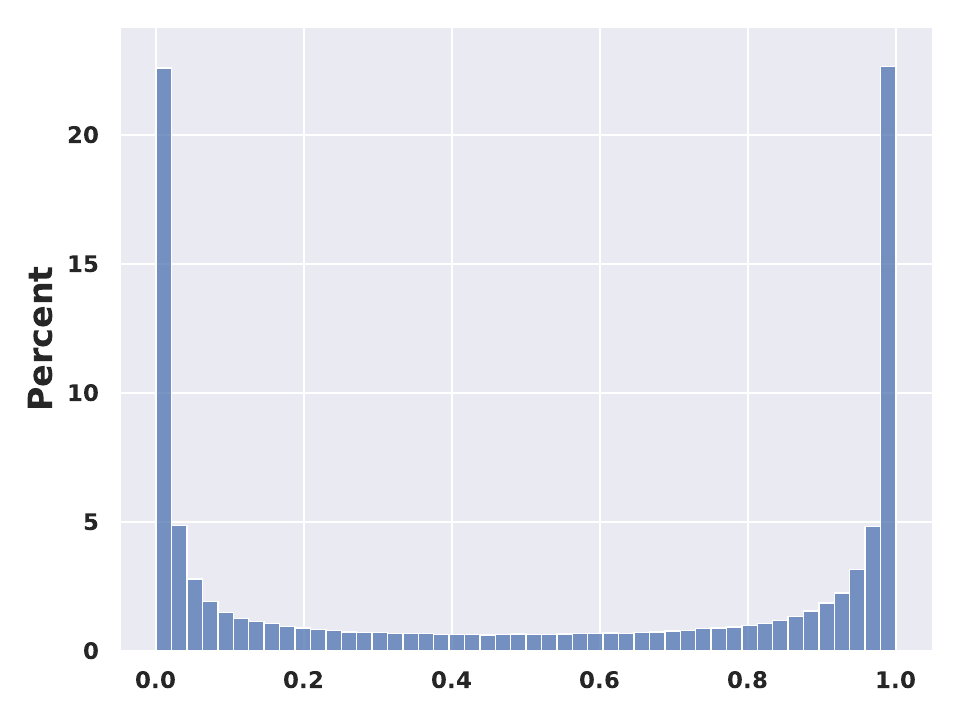}
		\caption{Class}
		\label{subfig: y_pred_train predict Class}
	\end{subfigure}
 	\begin{subfigure}{0.3\columnwidth}
        	\centering
		\includegraphics[width=\textwidth]{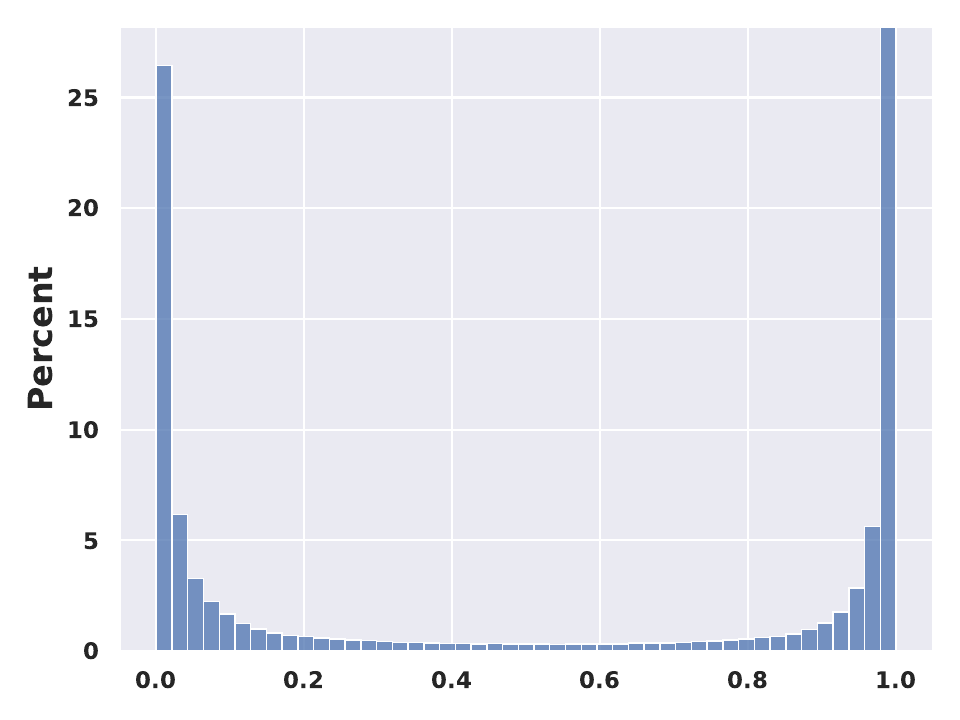}
		\caption{Family}
		\label{subfig: y_pred_train predict Family}
	\end{subfigure}
 	\begin{subfigure}{0.3\columnwidth}
        	\centering
		\includegraphics[width=\textwidth]{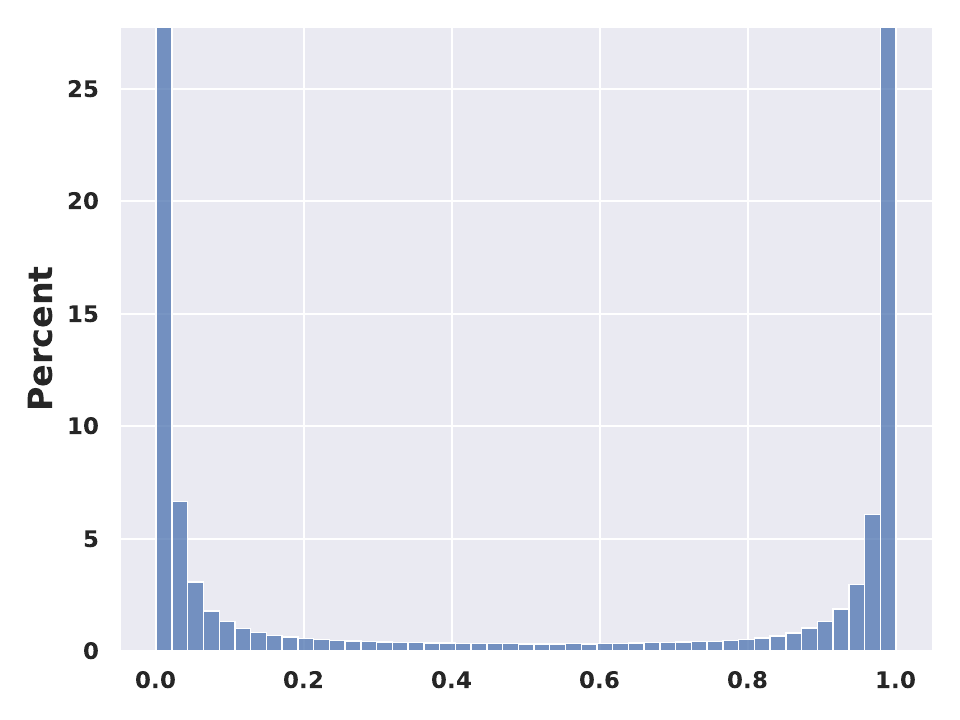}
		\caption{Genus}
		\label{subfig: y_pred_train predict Genus}
	\end{subfigure}
 	\begin{subfigure}{0.3\columnwidth}
        	\centering
		\includegraphics[width=\textwidth]{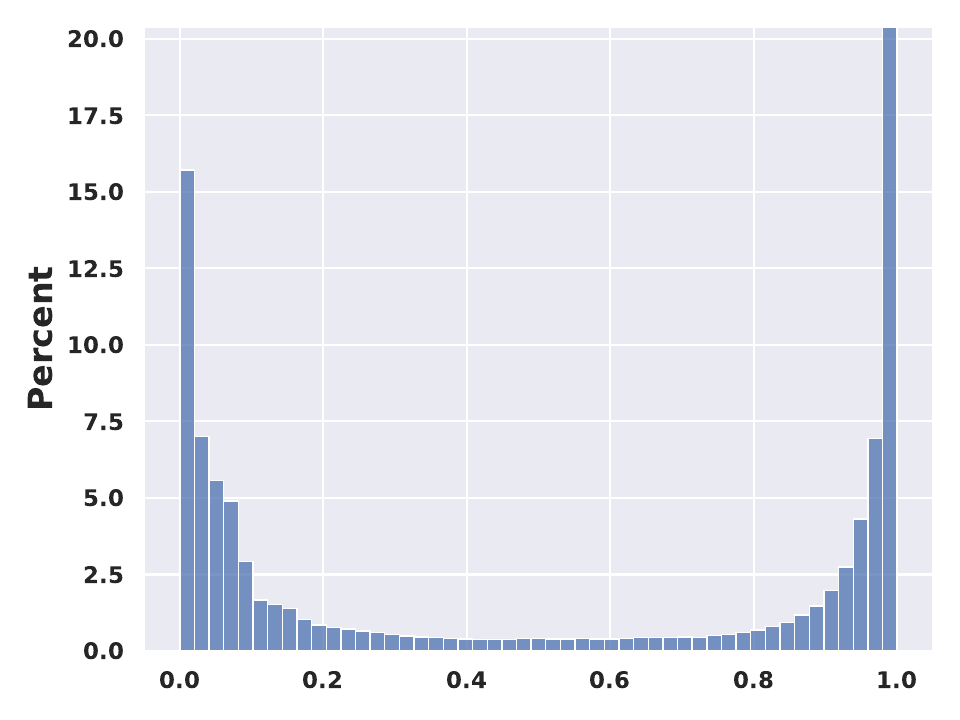}
		\caption{Species}
		\label{subfig: y_pred_train predict Species}
	\end{subfigure}
	\caption{Histogram of predicted probabilities on training data for different taxonomic ranks.}
	\label{fig: traing predicted probability}
\end{figure}

\begin{figure}[htbp]
	\centering
	\begin{subfigure}{0.3\columnwidth}
        	\centering
		\includegraphics[width=\textwidth]{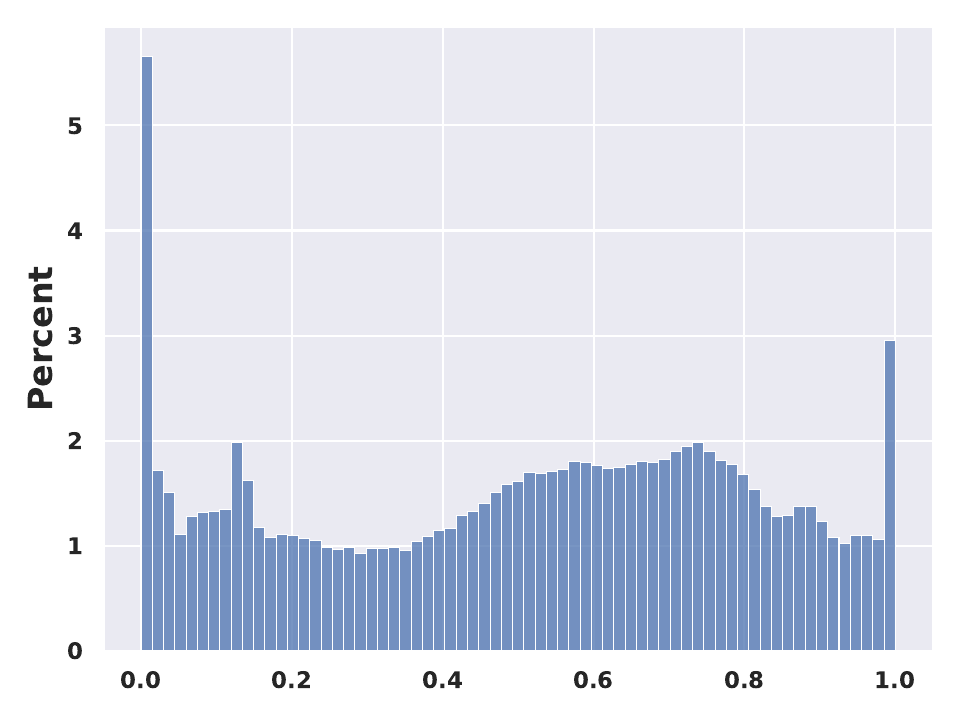}
		\caption{Kingdom}
		\label{subfig: y_pred_test predict Kingdom}
	\end{subfigure}
	\begin{subfigure}{0.3\columnwidth}
        	\centering
		\includegraphics[width=\textwidth]{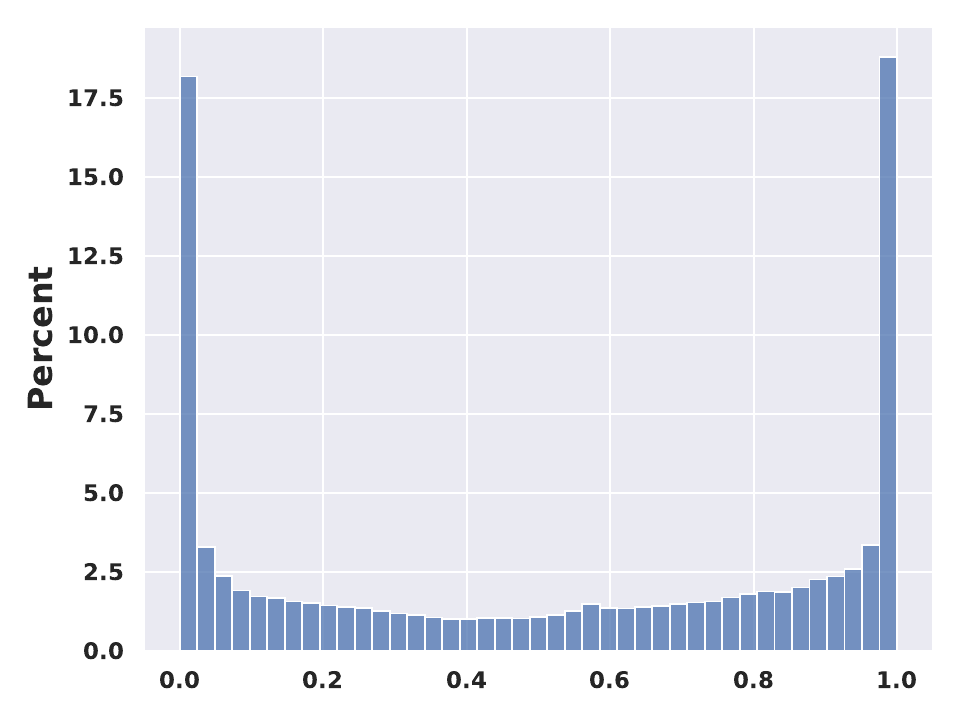}
		\caption{Phylum}
		\label{subfig: y_pred_test predict Phylum}
	\end{subfigure}
	\begin{subfigure}{0.3\columnwidth}
        	\centering
		\includegraphics[width=\textwidth]{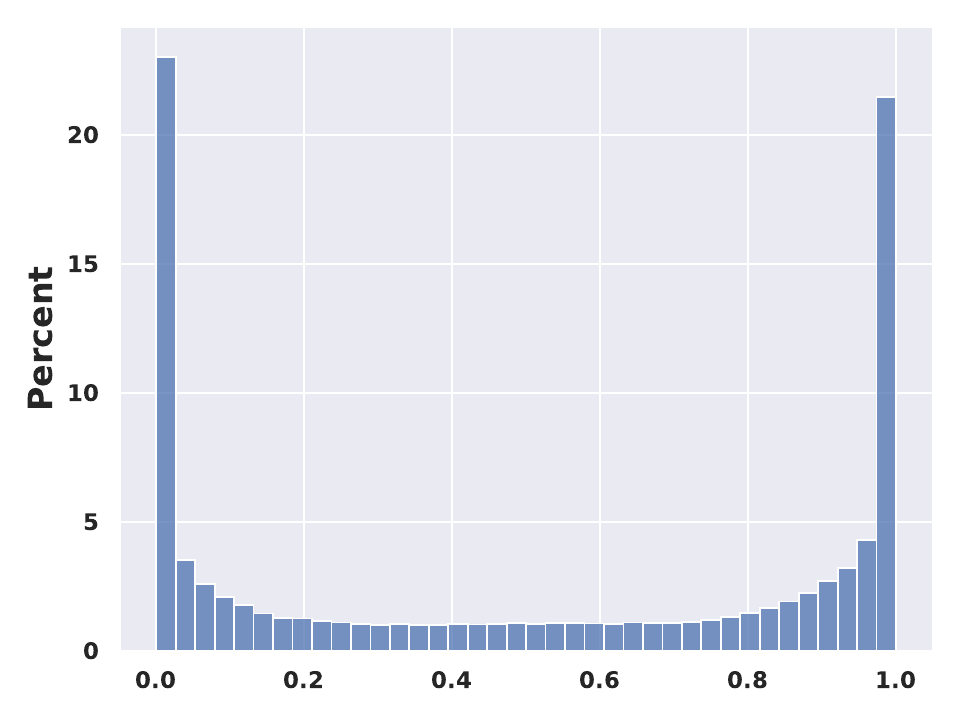}
		\caption{Class}
		\label{subfig: y_pred_test predict Class}
	\end{subfigure}
 	\begin{subfigure}{0.3\columnwidth}
        	\centering
		\includegraphics[width=\textwidth]{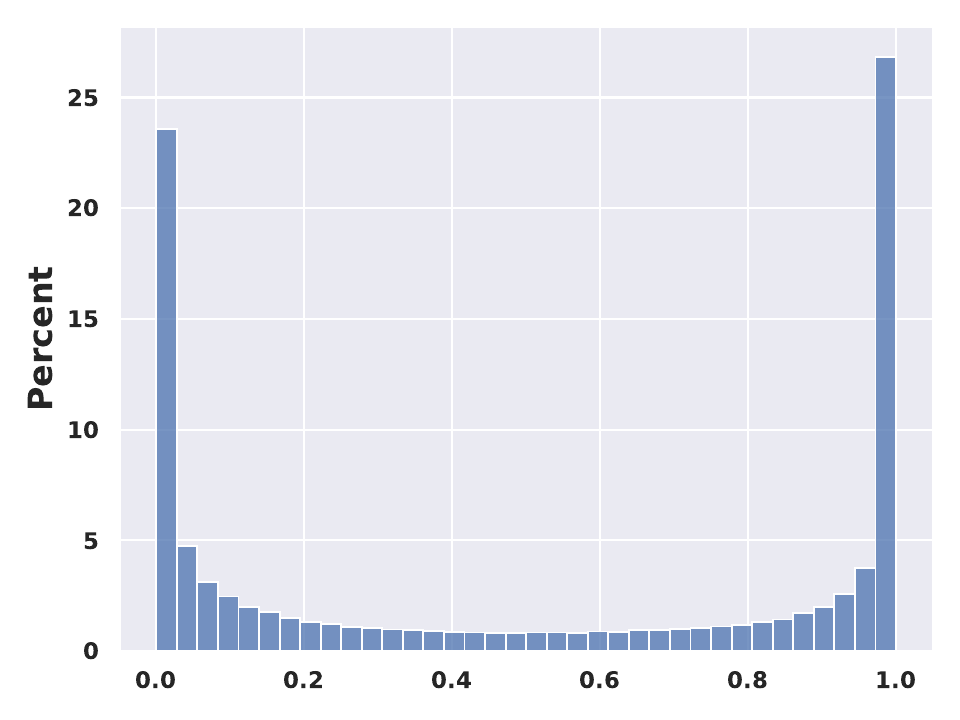}
		\caption{Family}
		\label{subfig: y_pred_test predict Family}
	\end{subfigure}
 	\begin{subfigure}{0.3\columnwidth}
        	\centering
		\includegraphics[width=\textwidth]{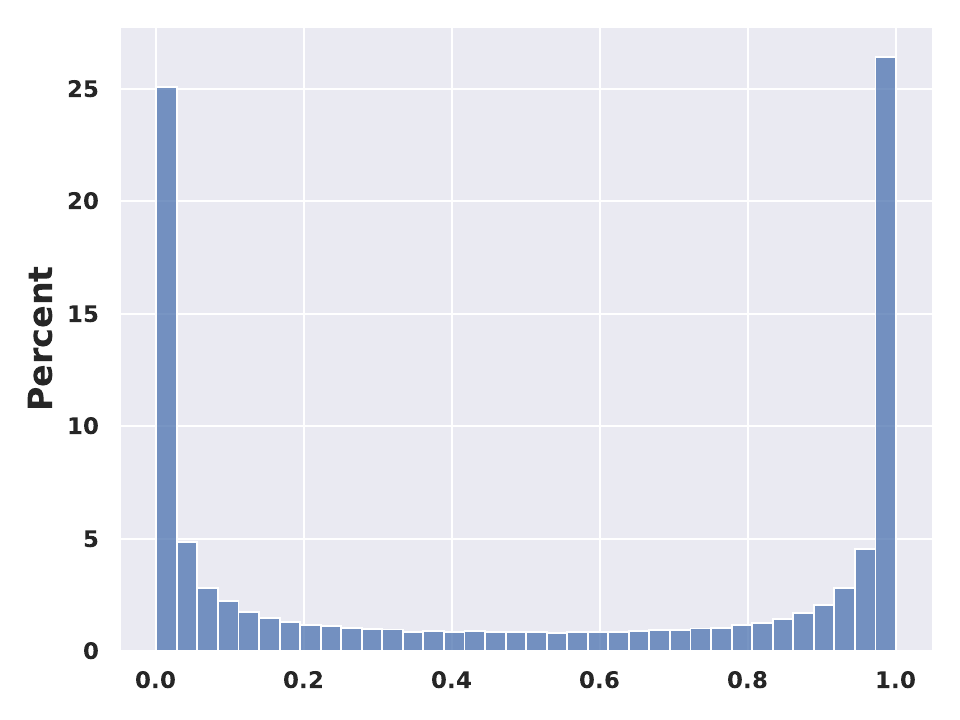}
		\caption{Genus}
		\label{subfig: y_pred_test predict Genus}
	\end{subfigure}
 	\begin{subfigure}{0.3\columnwidth}
        	\centering
		\includegraphics[width=\textwidth]{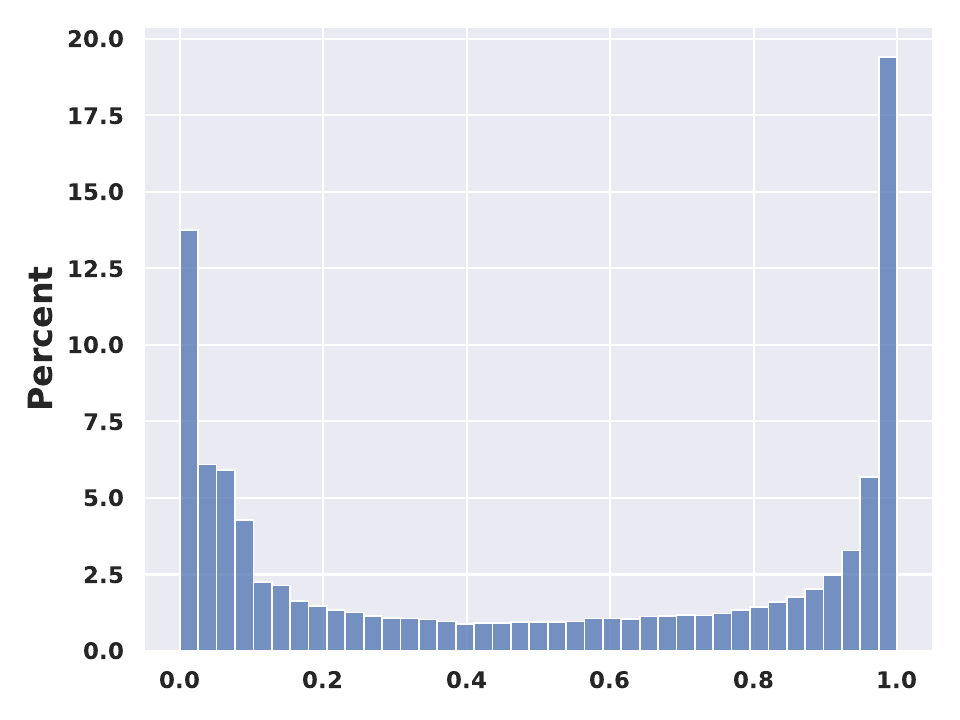}
		\caption{Species}
		\label{subfig: y_pred_test predict Species}
	\end{subfigure}
	\caption{Histogram of predicted probabilities on test data for different taxonomic ranks.}
	\label{fig: test predicted probability}
\end{figure}

\begin{figure}[htbp]
	\centering
	\begin{subfigure}{0.3\columnwidth}
        \centering
		\includegraphics[width=\textwidth]{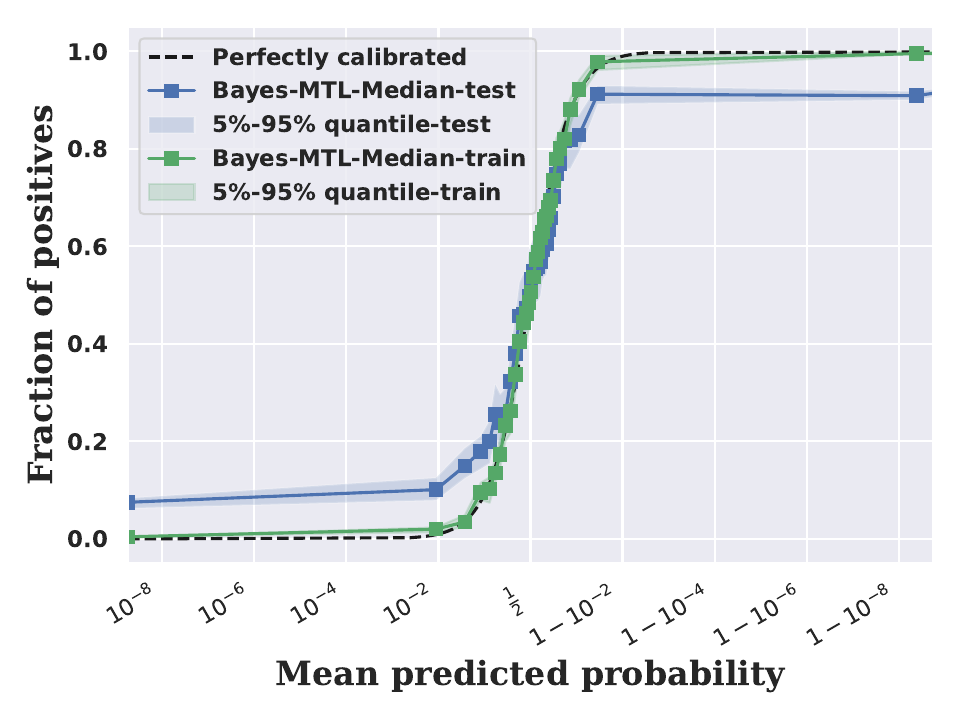}
		\caption{Kingdom}
	\end{subfigure}
	\begin{subfigure}{0.3\columnwidth}
        	\centering
		\includegraphics[width=\textwidth]{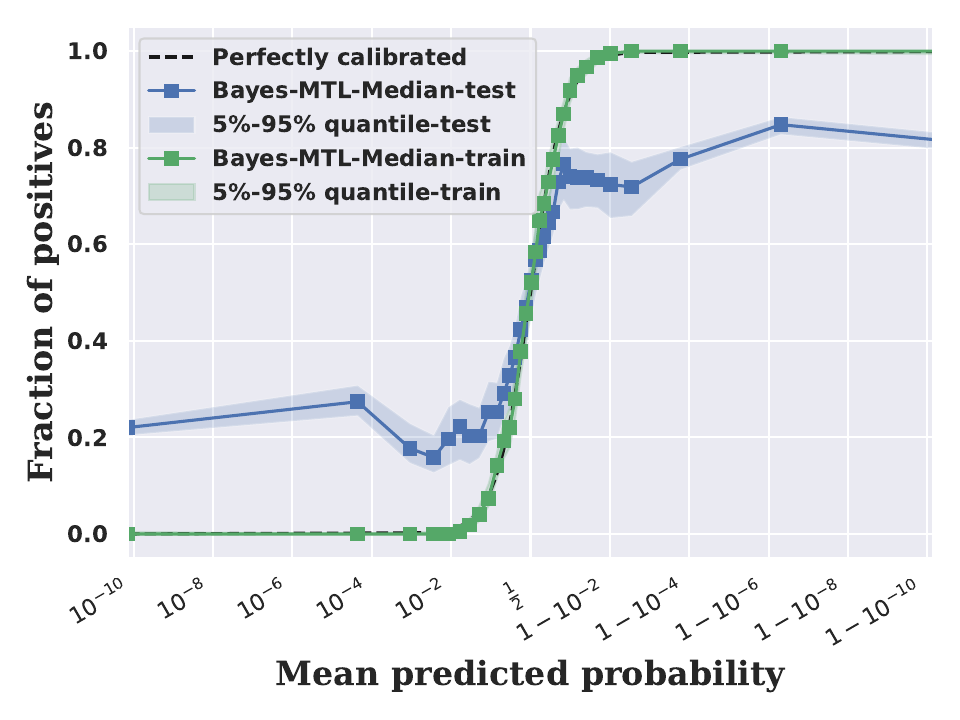}
		\caption{Phylum}
	\end{subfigure}
	\begin{subfigure}{0.3\columnwidth}
        	\centering
		\includegraphics[width=\textwidth]{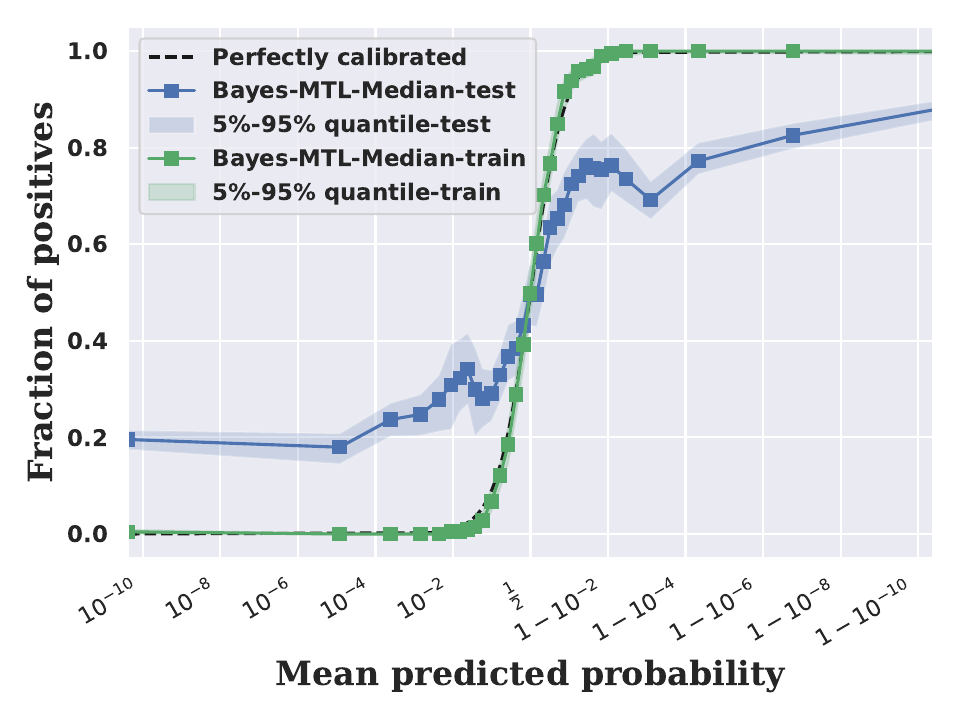}
		\caption{Class}
	\end{subfigure}
 	\begin{subfigure}{0.3\columnwidth}
        	\centering
		\includegraphics[width=\textwidth]{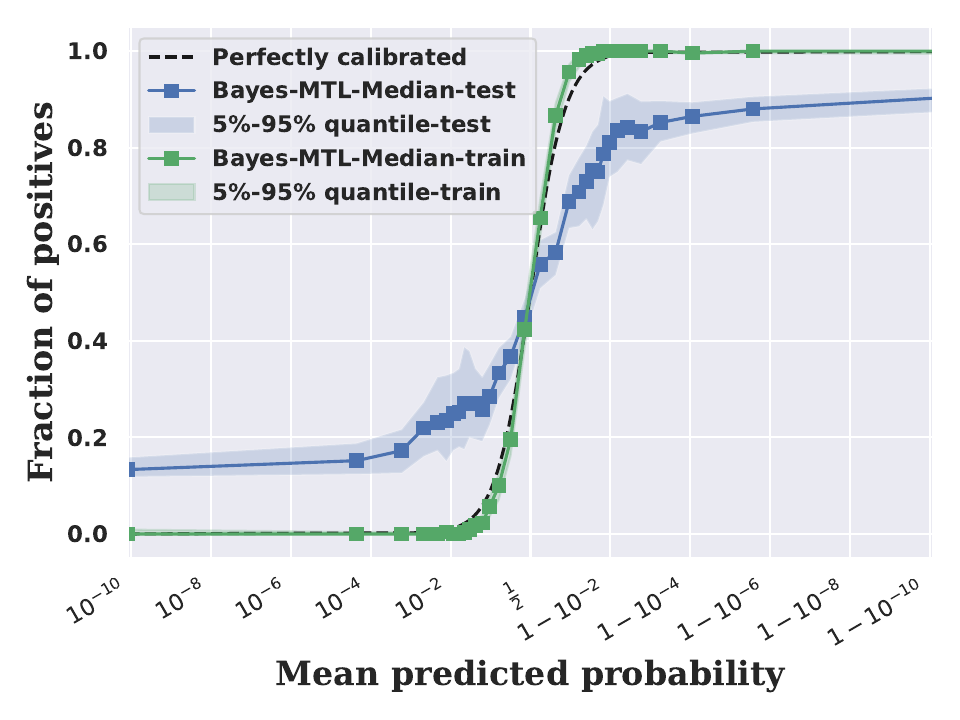}
		\caption{Family}
	\end{subfigure}
 	\begin{subfigure}{0.3\columnwidth}
        	\centering
		\includegraphics[width=\textwidth]{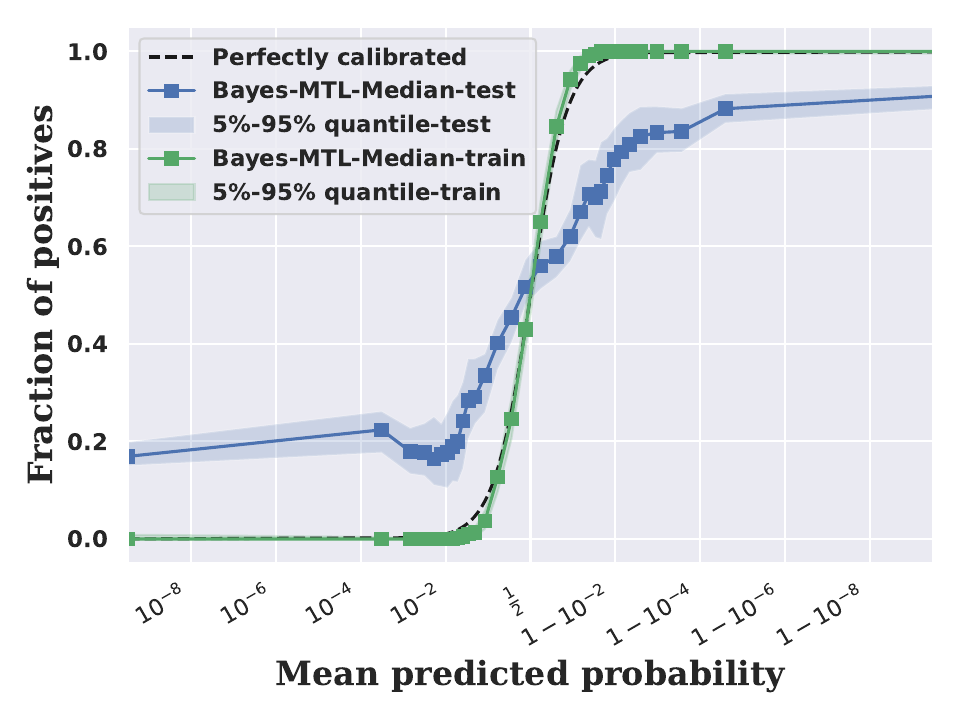}
		\caption{Genus}
	\end{subfigure}
 	\begin{subfigure}{0.3\columnwidth}
        	\centering
		\includegraphics[width=\textwidth]{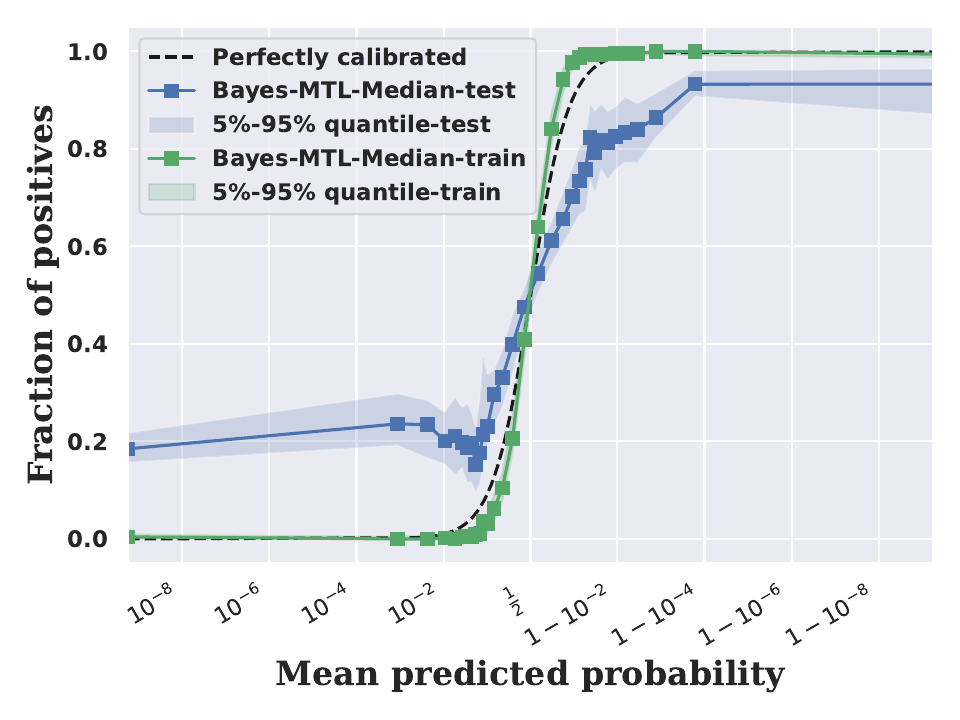}
		\caption{Species}
	\end{subfigure}
	\caption{Calibration curves for different taxonomic ranks.}
	\label{fig: calibration curves}
\end{figure}

\clearpage
\bibliographystyle{unsrt}
\bibliography{supp}
\end{document}
